# Supplementary material for: Exploring a Layer-Wise Design Space for KV Cache Eviction
Source: arXiv:2606.15157 source file (2026-09-17)
Supplement: Supplementary file 1 [file main.tex]

\section{Appendix}

\subsection{KV Cache Compression Taxonomy}

\begin{table}[t]
\centering
\footnotesize
\setlength{\tabcolsep}{3pt}
\begin{tabular}{@{}>{\raggedright\arraybackslash}p{0.23\linewidth}
>{\raggedright\arraybackslash}p{0.31\linewidth}
>{\raggedright\arraybackslash}p{0.18\linewidth}
>{\raggedright\arraybackslash}p{0.18\linewidth}@{}}
\hline
\textbf{Prior line} & \textbf{Main compression decision} & \textbf{Assignment axis} & \textbf{Budget axis} \\
\hline
H2O / Scissorhands & Attention-history or heavy-hitter eviction & Model-wide policy family & Fixed global budget \\
StreamingLLM & Sink tokens + recent window & Model-wide policy family & Fixed window and sink budget \\
Keyformer / SnapKV & Key-token or prompt-observation selection & Model-wide policy family & Uniform or default budget \\
KIVI / KVQuant & KV cache quantization & Model-wide quantization family & Quantization granularity or datatype, not cache-size allocation \\
KVMerger & Similarity-based KV state merging & Model-wide merge rule & Fixed compression ratio \\
FastGen & Head-profiled cache policy selection & Head-wise policy classes & Policy-dependent eviction \\
PyramidKV & Layer-wise cache-size schedule & Single selection family & Layer-wise budget \\
Ada-KV & Adaptive eviction budget & Single eviction family & Head-wise budget \\
DynamicKV & Task-aware adaptive eviction & Single eviction family & Layer-wise task-aware budget \\
LAVa & Information-loss-aware eviction & Single eviction family & Layer/head dynamic budget \\
RazorAttention / DuoAttention / HeadKV & Retrieval or important-head preservation & Head-wise policy classes & Head-wise cache allocation \\
LCKV / MiniCache & Depth-wise KV redundancy reduction & Layer/depth structural compression & Structural layer reduction \\
\textsc{PolyKV} & Heterogeneous method library & Layer- and phase-wise method assignment & Layer- and phase-wise budget allocation \\
\hline
\end{tabular}
\caption{Qualitative taxonomy of representative KV cache compression and sparse access methods along the two decisions studied in this work.
Earlier methods often instantiate one policy family across the model.
Recent adaptive methods show that cache capacity should vary across layers or heads, while head-profiled methods show that different heads can require different policies.
PolyKV targets the joint layer-wise choice of compression method and cache budget under a global memory constraint.}
\label{tab:baseline_taxonomy}
\end{table}

\subsection{Calibration Signals}

\begin{table}[t]
\centering
\small
\setlength{\tabcolsep}{3pt}
\begin{tabular}{@{}>{\raggedright\arraybackslash}p{0.17\linewidth}
>{\raggedright\arraybackslash}p{0.32\linewidth}
>{\raggedright\arraybackslash}p{0.20\linewidth}
>{\raggedright\arraybackslash}p{0.22\linewidth}@{}}
\hline
Signal & Definition & Decision & Intuition \\
\hline
Entropy &
$-\sum_k A^{(\ell,t)}_{h,q,k}\log A^{(\ell,t)}_{h,q,k}$ &
Budget allocation &
Diffuse attention suggests that more retained KV states may be useful. \\
\hline
Heavy-hitter ratio &
Top-$10\%$ key mass,
$\sum_{k \in \mathrm{TopK}(A_{h,q,:}^{(\ell,t)})} A^{(\ell,t)}_{h,q,k}$ &
Method selection &
Concentrated mass favors policies that preserve high-attention tokens. \\
\hline
Attention span &
Normalized attention-weighted lookback distance &
Method selection &
Long-range layers benefit from policies that preserve distant context. \\
\hline
Output cosine similarity &
Cosine similarity between full-cache and compressed layer outputs &
Method selection &
High similarity indicates that a candidate preserves the layer computation. \\
\hline
PPL sensitivity &
Increase in calibration perplexity after applying a candidate to a layer-phase
slot &
Method selection and budget allocation &
Sensitive layers should receive safer methods or larger budgets. \\
\hline
\end{tabular}
\caption{Calibration signals used to instantiate the PolyKV plan.
Signals are computed offline and converted into fixed per-layer, per-phase decisions.}
\label{tab:polykv_signals}
\end{table}

\subsection{Full Signal Validation Table}

\input{assets/table/signal_validation_results}

\subsection{Completed LongBench Budget Sweep}
\label{app:longbench_budget_sweep}

\begin{table}[t]
\centering
\small
\setlength{\tabcolsep}{3.4pt}
\resizebox{\linewidth}{!}{%
\begin{tabular}{@{}c l r r r r r r@{}}
\hline
Budget & Best single & Route only & Uniform combo & PPL-budget combo &
Best PolyKV & Gain & PPL combo gap closed \\
\hline
128 & TOVA 33.59 & 35.75 & 35.74 & 35.44 & 35.75 & +2.16 & 34.2\% \\
256 & CAKE 34.62 & 36.84 & 36.85 & 36.67 & 36.85 & +2.22 & 46.9\% \\
512 & Quest 36.55 & 37.59 & 37.60 & 37.79 & 37.79 & +1.24 & 51.0\% \\
768 & Quest 37.08 & 37.87 & 37.87 & 38.08 & 38.08 & +1.00 & 52.6\% \\
1024 & CAKE 37.57 & 38.03 & 38.03 & 38.22 & 38.22 & +0.65 & 45.8\% \\
\hline
\end{tabular}
}
\caption{Llama-3.1-8B-Instruct LongBench scores under fixed KV budgets.
``Gain'' compares the best completed PolyKV score with the best completed single-method baseline at the same budget.
``PPL combo gap closed'' is computed for the named PPL-budget combo against the same best-single baseline and the full-cache score of 38.99; at budgets 128 and 256, route-only or uniform-combo variants are the best completed PolyKV rows.}
\label{tab:main_longbench_results}
\end{table}

\begin{figure}[t]
\centering
\includegraphics[width=0.92\linewidth]{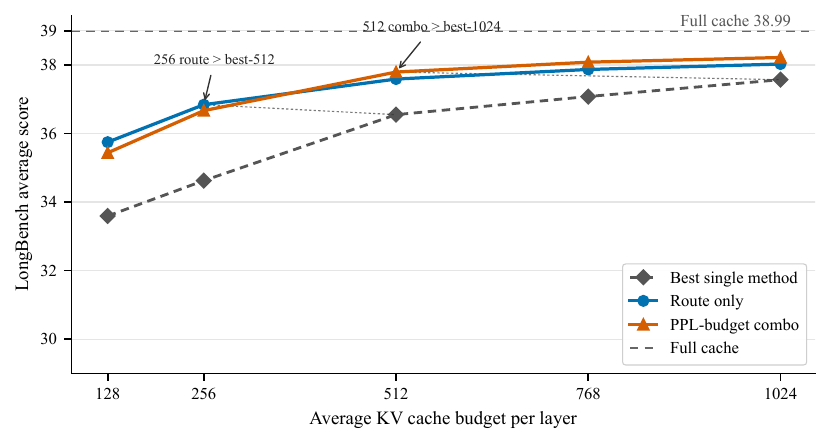}
\caption{LongBench budget scaling for the best completed single-method baseline and two named PolyKV configurations.
Route-only uses layer-wise method selection with a uniform budget; PPL-budget combo additionally applies signal-guided budget allocation.
The dashed line shows full-cache performance.}
\label{fig:longbench_budget_scaling}
\end{figure}

\begin{figure}[t]
\centering
\includegraphics[width=\linewidth]{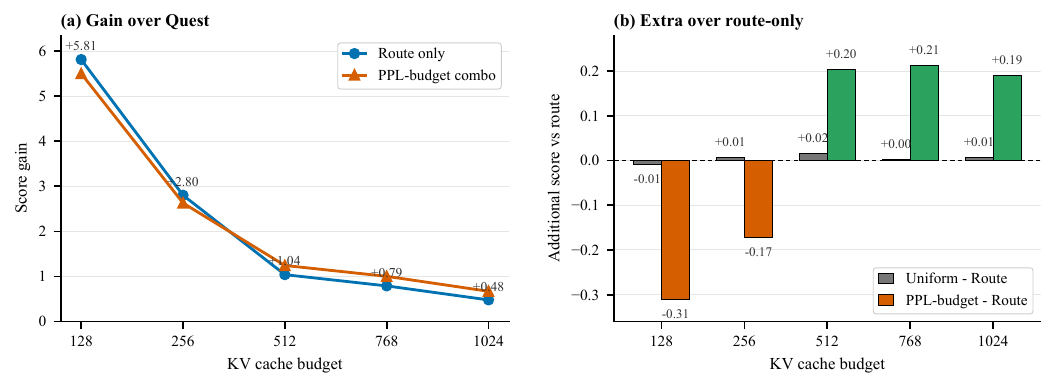}
\caption{Ablation decomposition at matched KV cache budgets.
Panel (a) reports score gains over Quest, and panel (b) reports the additional gain of PPL-sensitivity budget allocation over route-only.}
\label{fig:polykv_ablation_decomposition}
\end{figure}

\subsection{Policy and Cross-Model Diagnostics}
\label{app:policy_cross_model_diagnostics}

\begin{figure}[t]
\centering
\includegraphics[width=\linewidth]{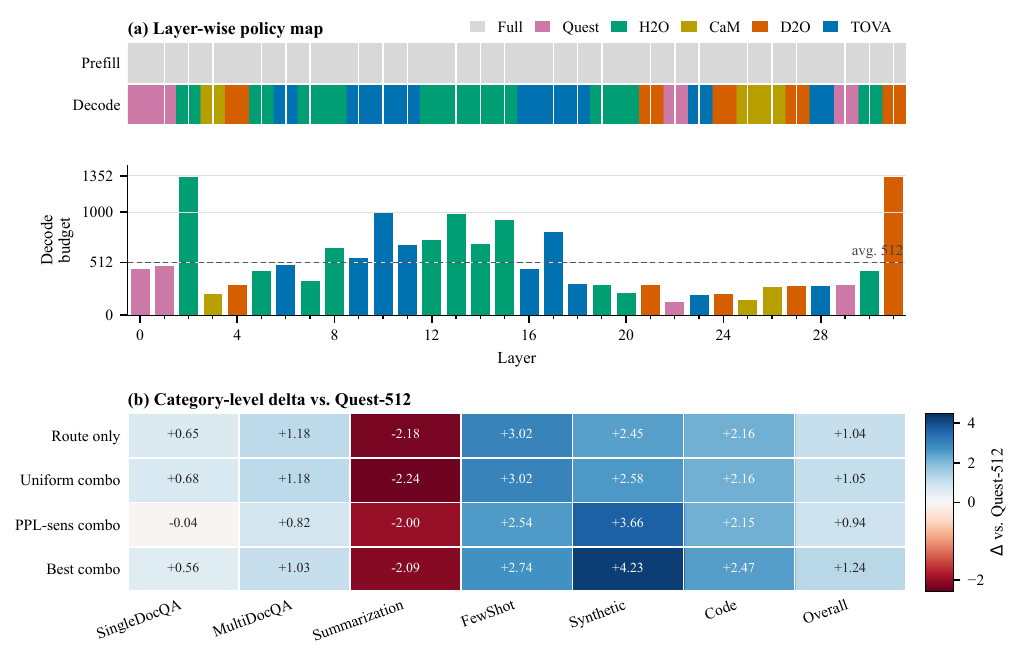}
\caption{Policy and category analysis at budget 512.
(a) A representative heterogeneous policy keeps prefill full, routes decode layers across multiple compression methods, and assigns non-uniform decode budgets across layers.
(b) Category-level LongBench deltas for 512-budget heterogeneous configurations are computed against Quest-512.}
\label{fig:policy_category_maps_512}
\end{figure}

\begin{table}[t]
\centering
\small
\setlength{\tabcolsep}{3.6pt}
\resizebox{\linewidth}{!}{%
\begin{tabular}{@{}l l l l r@{}}
\hline
Model & Benchmark & Baseline & PolyKV configuration & Gain \\
\hline
Llama-3.1-8B & LongBench & Quest 36.55 &
\texttt{combo\_ppl\_sens\_cosine\_decode} 37.79 & +1.24 \\
Llama-3.1-8B & RULER & TOVA 58.54 &
\texttt{route\_cosine\_both} 58.91 & +0.37 \\
Qwen3-8B & LongBench & CAKE 47.01 &
\texttt{combo\_uniform\_ppl\_sens\_decode} 47.54 & +0.54 \\
Qwen3-8B & RULER & CAKE 55.59 &
\texttt{var\_entropy\_snapkv} 51.61 & -3.98 \\
\hline
\end{tabular}
}
\caption{512-budget comparison across models and benchmarks.
LongBench rows compare against the best completed single-method baseline and select the best completed PolyKV combo configuration.
RULER rows use the best completed eviction baseline, excluding Quest because it is not an eviction method, and select the best completed PolyKV configuration under that protocol.}
\label{tab:cross_model_512_summary}
\end{table}

\subsection{Configuration Rankings and Signal Pattern Diagnostics}
\label{app:configuration_diagnostics}

\begin{figure}[t]
\centering
\includegraphics[width=\linewidth]{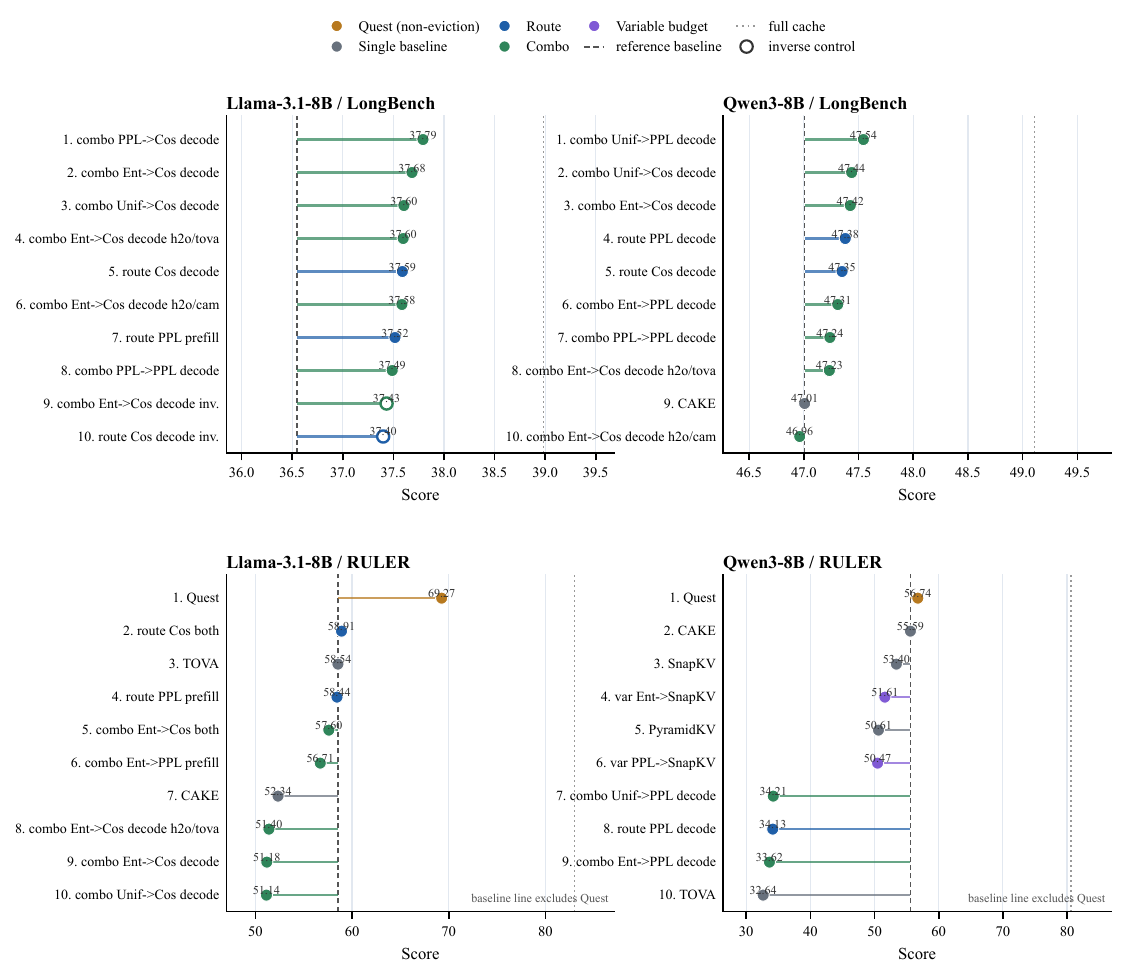}
\caption{Top 512-budget configuration rankings across models and benchmarks.
Dashed vertical lines mark the reference baseline used for the gain calculation: the best completed single-method baseline on LongBench and the best completed eviction baseline on RULER.
Quest is shown separately on RULER because it is not an eviction method.
Dotted lines mark full-cache performance.
Hollow markers denote inverse-control configurations.}
\label{fig:config_ranking_patterns_512}
\end{figure}

\begin{figure}[t]
\centering
\includegraphics[width=0.76\linewidth]{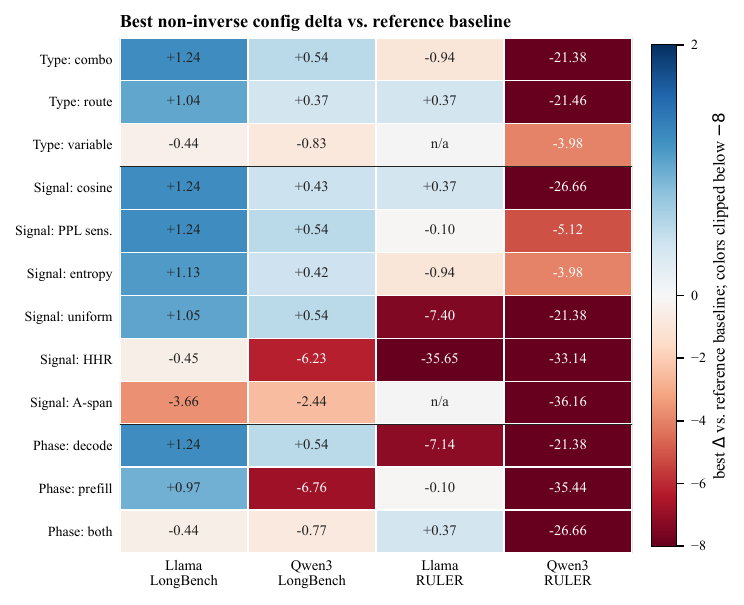}
\caption{Signal and stage summary for 512-budget non-inverse PolyKV configurations, excluding single-method baselines and full-cache runs.
Each cell reports the best observed score delta over the same reference baseline used in Figure~\ref{fig:config_ranking_patterns_512}.
Colors are clipped below $-8$ points so that small positive LongBench differences remain visible.
Empty cells indicate unavailable configurations.}
\label{fig:config_signal_pattern_summary_512}
\end{figure}

\subsection{Task and Length Diagnostics}
\label{app:task_length_diagnostics}

\begin{table}[t]
\centering
\scriptsize
\setlength{\tabcolsep}{3pt}
\begin{tabular}{@{}l r r r r r r r@{}}
\hline
Length bin & Count & Quest-512 & Ours-512 & $\Delta$ Score &
Quest hit & Ours hit & $\Delta$ Hit \\
\hline
0--2k & 790 & 50.20 & 51.28 & +1.08 & 97.47 & 97.72 & +0.25 \\
2--4k & 759 & 37.08 & 37.33 & +0.25 & 91.04 & 91.31 & +0.26 \\
4--6k & 582 & 38.13 & 38.56 & +0.43 & 86.60 & 86.77 & +0.17 \\
6--8k & 616 & 49.01 & 52.06 & +3.04 & 87.66 & 88.15 & +0.49 \\
8--10k & 568 & 49.02 & 50.26 & +1.24 & 86.62 & 86.09 & -0.53 \\
10--12k & 537 & 26.61 & 27.17 & +0.56 & 71.51 & 73.93 & +2.42 \\
12--14k & 256 & 27.03 & 26.67 & -0.36 & 72.66 & 71.48 & -1.18 \\
14--16k & 162 & 28.67 & 28.07 & -0.60 & 75.93 & 75.93 & -0.00 \\
16--18k & 99 & 21.84 & 23.41 & +1.57 & 74.74 & 73.74 & -1.01 \\
$\geq18$k original, truncated & 381 & 24.22 & 30.85 & +6.63 &
70.34 & 75.59 & +5.25 \\
\hline
\end{tabular}
\caption{Full length-conditioned diagnostic at budget 512.
Score and hit-rate values are computed within each original length bin.}
\label{tab:length_conditioned_delta_full}
\end{table}

\begin{figure}[t]
\centering
\includegraphics[width=\linewidth]{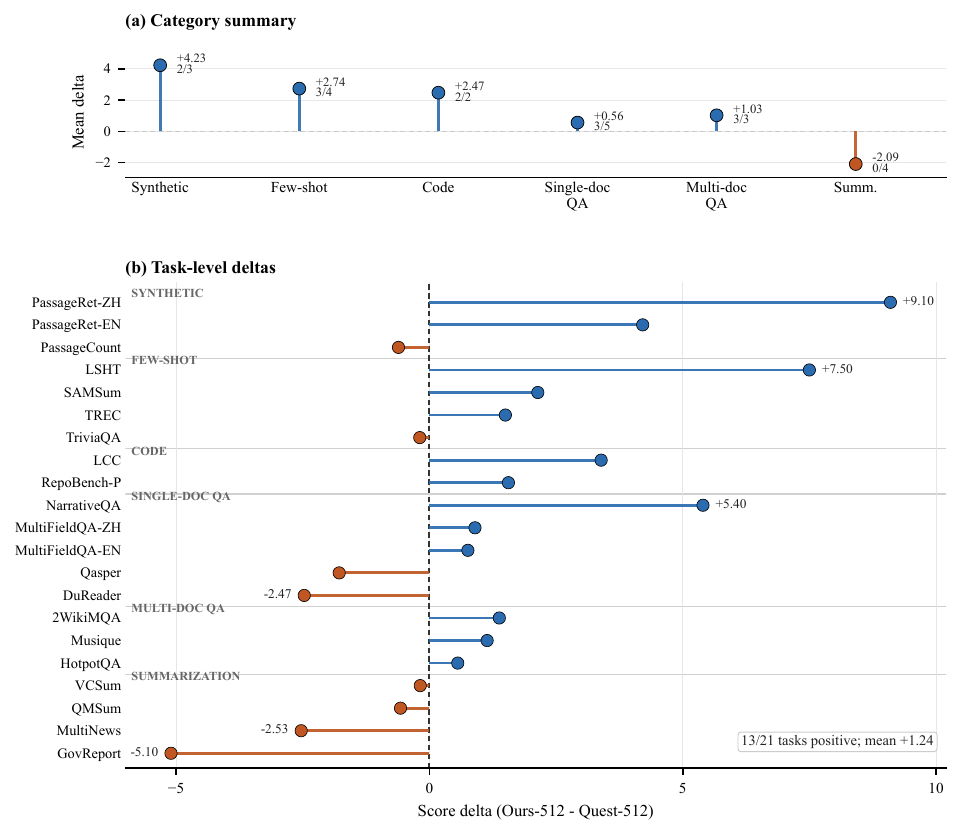}
\caption{Per-task score deltas between Ours-512 and Quest-512 on LongBench.}
\label{fig:task_delta_waterfall_quest512_vs_ours512}
\end{figure}

\begin{figure}[t]
\centering
\includegraphics[width=\linewidth]{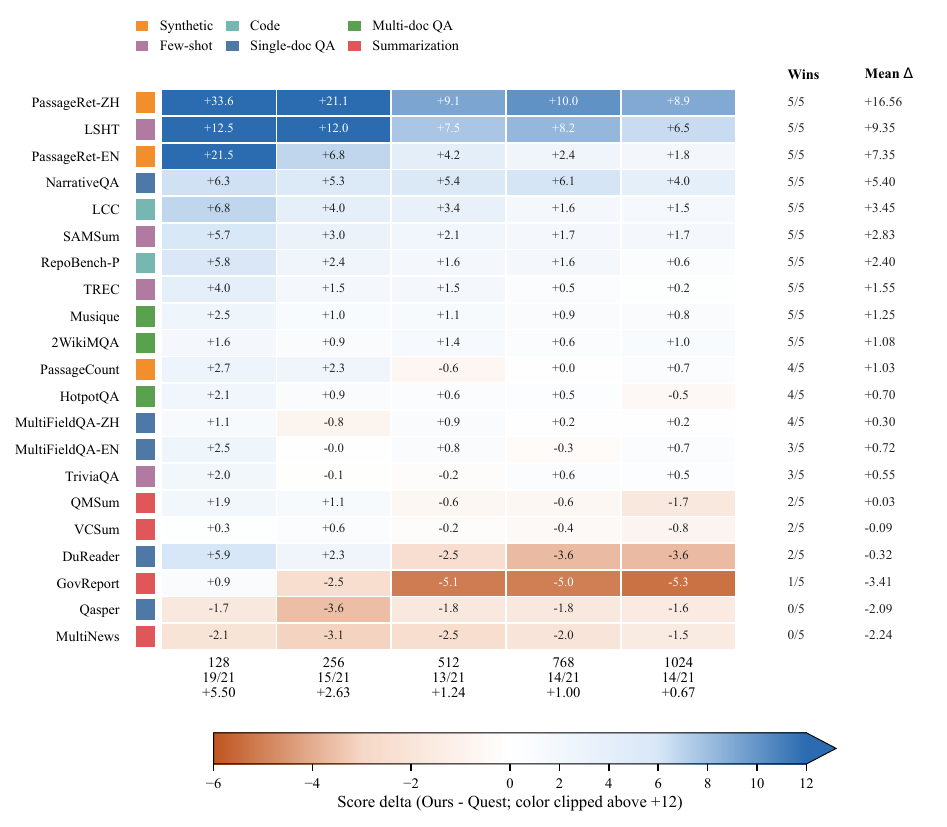}
\caption{Task-level score deltas between PolyKV and Quest across matched budgets.
Positive cells indicate tasks where PolyKV improves over Quest.}
\label{fig:task_win_frequency_heatmap}
\end{figure}

\begin{figure}[t]
\centering
\includegraphics[width=\linewidth]{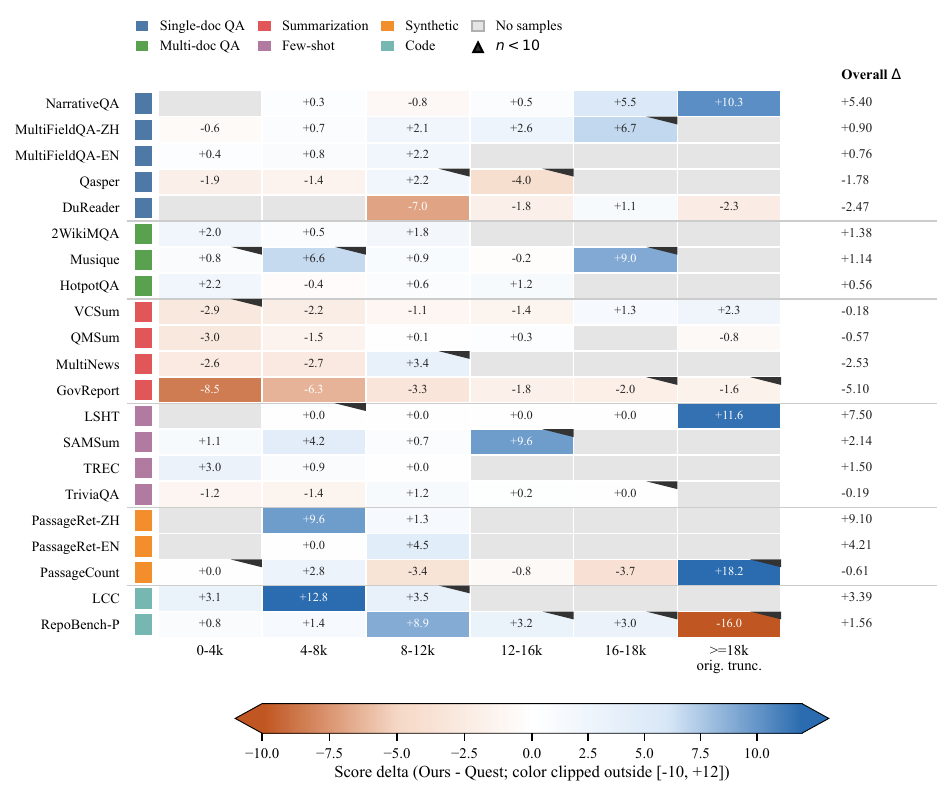}
\caption{Task-by-length diagnostic at budget 512.
Each cell shows the count-weighted score delta between PolyKV and Quest within an original-input-length bin.
Cells marked with a triangle have fewer than 10 samples.
Inputs above 18k original tokens are truncated before inference and grouped separately.}
\label{fig:task_length_delta_heatmap_quest512_vs_ours512}
\end{figure}

\subsection{Statistical Credibility and Full-Cache Recovery}
\label{app:statistical_recovery}

\begin{figure}[t]
\centering
\includegraphics[width=\linewidth]{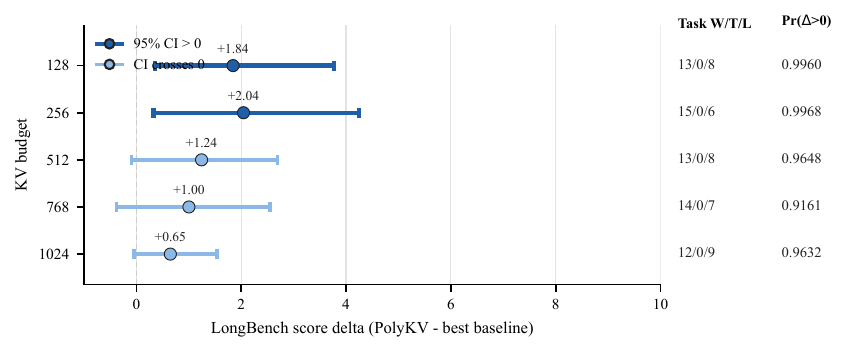}
\caption{Task-level paired bootstrap confidence intervals for PolyKV gains over the same-budget best single-method baseline.
Each bootstrap sample resamples the 21 LongBench tasks with replacement and recomputes the macro-average score delta.}
\label{fig:statistical_credibility_polykv_gains}
\end{figure}

\begin{figure}[t]
\centering
\includegraphics[width=\linewidth]{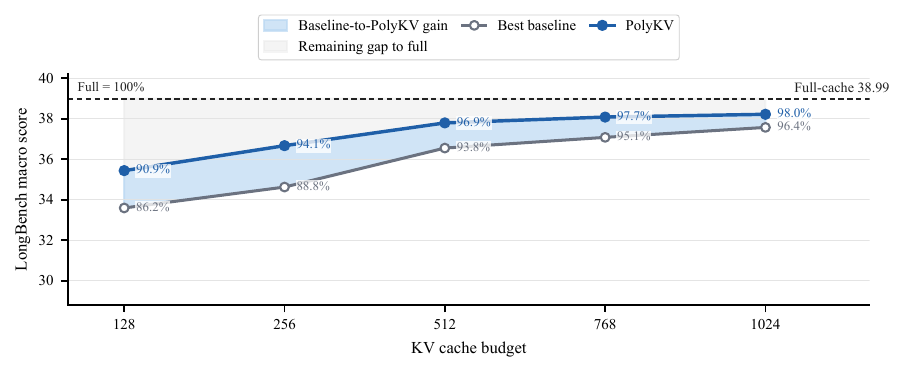}
\caption{Full-cache recovery on the 21-task LongBench macro average.
The horizontal line marks the full-cache score; point labels report each method's score as a percentage of the full-cache score.}
\label{fig:full_cache_recovery_gap_to_full}
\end{figure}

\subsection{Complete LongBench and RULER results}

\begin{table}[t]
\centering
\small
\setlength{\tabcolsep}{4.2pt}
\resizebox{\linewidth}{!}{%
\begin{tabular}{@{}lrrrr@{}}
\toprule
Method & Llama LongBench & Qwen LongBench & Llama RULER & Qwen RULER \\
\midrule
Full cache & 38.9857 & 49.1095 & 83.0100 & 80.6400 \\
\midrule
CAKE & 36.3514 & 47.0071 & 52.3400 & 55.5900 \\
SnapKV & 35.9352 & 46.6133 & 42.4600 & 53.4000 \\
PyramidKV & 35.8090 & 45.8057 & 48.9100 & 50.6100 \\
TOVA & 35.6962 & 45.9043 & 58.5400 & 32.6400 \\
H2O & 32.7910 & 39.8705 & 17.2100 & 16.9800 \\
CaM & 32.7248 & 40.1052 & 17.1900 & 16.9800 \\
ScissorHands & 31.1881 & 38.0843 & 18.3300 & 16.8700 \\
StreamingLLM & 15.8124 & 10.0714 & 3.7500 & 2.3100 \\
D2O & 11.6457 & 3.5005 & 0.3100 & 1.3100 \\
\bottomrule
\end{tabular}
}
\caption{Complete 512-budget single-method scores used for the coarse comparison.
LongBench reports the 21-task macro average, and RULER reports the global average; higher is better.
Quest is shown for completeness but excluded from the best-eviction-single baseline because it is not an eviction method.}
\label{tab:appendix_512_single_methods}
\end{table}

\begin{table}[t]
\centering
\scriptsize
\setlength{\tabcolsep}{3.2pt}
\resizebox{\linewidth}{!}{%
\begin{tabular}{@{}llrr@{}}
\toprule
Model / benchmark & Rank & Score & Short label \\
\midrule
Llama LongBench & 1 & 37.7929 &
PPL budget + cosine decode \\
Llama LongBench & 2 & 37.6843 &
entropy budget + cosine decode \\
Llama LongBench & 3 & 37.6043 &
uniform + cosine decode \\
Llama LongBench & 4 & 37.5971 &
entropy + restricted cosine decode \\
Llama LongBench & 5 & 37.5890 &
route-only cosine decode \\
\midrule
Qwen LongBench & 1 & 47.5443 &
uniform + PPL decode \\
Qwen LongBench & 2 & 47.4371 &
uniform + cosine decode \\
Qwen LongBench & 3 & 47.4243 &
entropy budget + cosine decode \\
Qwen LongBench & 4 & 47.3786 &
route-only PPL decode \\
Qwen LongBench & 5 & 47.3490 &
route-only cosine decode \\
\midrule
Llama RULER & 1 & 58.9100 &
route-only cosine both \\
Llama RULER & 2 & 58.4400 &
route-only PPL prefill \\
Llama RULER & 3 & 57.6000 &
entropy + cosine both \\
Llama RULER & 4 & 56.7100 &
entropy + PPL prefill \\
Llama RULER & 5 & 51.4000 &
entropy + restricted cosine decode \\
\midrule
Qwen RULER & 1 & 51.6100 &
entropy budget + fixed SnapKV \\
Qwen RULER & 2 & 50.4700 &
PPL budget + fixed SnapKV \\
Qwen RULER & 3 & 34.2100 &
uniform + PPL decode \\
Qwen RULER & 4 & 34.1300 &
route-only PPL decode \\
Qwen RULER & 5 & 33.6200 &
entropy + PPL decode \\
\bottomrule
\end{tabular}
}
\caption{Top-5 completed PolyKV configurations at budget 512.
These rows define the completed-configuration envelope used in the coarse main-text comparison; they should not be interpreted as one fixed default PolyKV policy.}
\label{tab:appendix_512_polykv_top5}
\end{table}

\subsection{All result of budget sweep}

\begin{table}[t]
\centering
\small
\setlength{\tabcolsep}{4.2pt}
\resizebox{\linewidth}{!}{%
\begin{tabular}{@{}lrrrrr@{}}
\toprule
Method / configuration & 128 & 256 & 512 & 768 & 1024 \\
\midrule
Full cache & \multicolumn{5}{c}{38.9857} \\
\midrule
\multicolumn{6}{@{}l}{\textit{Single baselines}} \\
CAKE & 32.1214 & 34.6248 & 36.3514 & 36.9890 & 37.5705 \\
CaM & 29.5862 & 31.4490 & 32.7248 & 33.9633 & 34.5600 \\
D2O & 11.9476 & 11.5695 & 11.6457 & 11.9238 & 11.8486 \\
H2O & 29.0733 & 31.3352 & 32.7910 & 33.9533 & 34.7167 \\
PyramidKV & 31.7910 & 34.1567 & 35.8090 & 36.6376 & 37.1414 \\
ScissorHands & 27.1529 & 29.2233 & 31.1881 & 32.0886 & 33.2905 \\
SnapKV & 32.2457 & 34.5805 & 35.9352 & 36.5167 & 36.9905 \\
StreamingLLM & 17.6043 & 16.8233 & 15.8124 & 15.5871 & 15.1319 \\
TOVA & 33.5924 & 34.4814 & 35.6962 & 36.4300 & 37.0571 \\
\midrule
\multicolumn{6}{@{}l}{\textit{PolyKV budget sweep variants}} \\
Method selection only & 35.7476 & 36.8410 & 37.5890 & 37.8690 & 38.0267 \\
Method selection w/ budget allocation & 35.4362 & 36.6681 & 37.7929 & 38.0814 & 38.2181 \\
\bottomrule
\end{tabular}
}
\caption{Complete Llama-3.1-8B-Instruct LongBench budget sweep.
Scores are 21-task macro averages from raw LongBench outputs; higher is better.
Full cache is budget-free and shown once.
Quest is included for completeness but marked as non-eviction.
Method selection only uses \texttt{cosine\_decode} routing with a uniform per-layer budget; Method selection w/ budget allocation keeps the same routing but assigns a non-uniform PPL-sensitivity budget scaled to the target average budget.
Uniform-budget combo is the combo-schema uniform-budget control.}
\label{tab:appendix_llama_longbench_budget_sweep_matrix}
\end{table}
