# Supplementary material for: Exploring a Layer-Wise Design Space for KV Cache Eviction
Source: arXiv:2606.15157 source file (2026-09-17)
Supplement: Supplementary file 2 [file appendix_512_polykv_top5.tex]

\begin{table}[t]
\centering
\scriptsize
\setlength{\tabcolsep}{3.2pt}
\resizebox{\linewidth}{!}{%
\begin{tabular}{@{}llrr@{}}
\toprule
Model / benchmark & Rank & Score & Short label \\
\midrule
Llama LongBench & 1 & 37.7929 &
PPL budget + cosine decode \\
Llama LongBench & 2 & 37.6843 &
entropy budget + cosine decode \\
Llama LongBench & 3 & 37.6043 &
uniform + cosine decode \\
Llama LongBench & 4 & 37.5971 &
entropy + restricted cosine decode \\
Llama LongBench & 5 & 37.5890 &
route-only cosine decode \\
\midrule
Qwen LongBench & 1 & 47.5443 &
uniform + PPL decode \\
Qwen LongBench & 2 & 47.4371 &
uniform + cosine decode \\
Qwen LongBench & 3 & 47.4243 &
entropy budget + cosine decode \\
Qwen LongBench & 4 & 47.3786 &
route-only PPL decode \\
Qwen LongBench & 5 & 47.3490 &
route-only cosine decode \\
\midrule
Llama RULER & 1 & 58.9100 &
route-only cosine both \\
Llama RULER & 2 & 58.4400 &
route-only PPL prefill \\
Llama RULER & 3 & 57.6000 &
entropy + cosine both \\
Llama RULER & 4 & 56.7100 &
entropy + PPL prefill \\
Llama RULER & 5 & 51.4000 &
entropy + restricted cosine decode \\
\midrule
Qwen RULER & 1 & 51.6100 &
entropy budget + fixed SnapKV \\
Qwen RULER & 2 & 50.4700 &
PPL budget + fixed SnapKV \\
Qwen RULER & 3 & 34.2100 &
uniform + PPL decode \\
Qwen RULER & 4 & 34.1300 &
route-only PPL decode \\
Qwen RULER & 5 & 33.6200 &
entropy + PPL decode \\
\bottomrule
\end{tabular}
}
\caption{Top-5 completed PolyKV configurations at budget 512.
These rows define the completed-configuration envelope used in the coarse main-text comparison; they should not be interpreted as one fixed default PolyKV policy.}
\label{tab:appendix_512_polykv_top5}
\end{table}
