# Supplementary material for: Exploring a Layer-Wise Design Space for KV Cache Eviction
Source: arXiv:2606.15157 source file (2026-09-17)
Supplement: Supplementary file 3 [file appendix_512_single_methods.tex]

\begin{table}[t]
\centering
\small
\setlength{\tabcolsep}{4.2pt}
\resizebox{\linewidth}{!}{%
\begin{tabular}{@{}lrrrr@{}}
\toprule
Method & Llama LongBench & Qwen LongBench & Llama RULER & Qwen RULER \\
\midrule
Full cache & 38.9857 & 49.1095 & 83.0100 & 80.6400 \\
\midrule
CAKE & 36.3514 & 47.0071 & 52.3400 & 55.5900 \\
SnapKV & 35.9352 & 46.6133 & 42.4600 & 53.4000 \\
PyramidKV & 35.8090 & 45.8057 & 48.9100 & 50.6100 \\
TOVA & 35.6962 & 45.9043 & 58.5400 & 32.6400 \\
H2O & 32.7910 & 39.8705 & 17.2100 & 16.9800 \\
CaM & 32.7248 & 40.1052 & 17.1900 & 16.9800 \\
ScissorHands & 31.1881 & 38.0843 & 18.3300 & 16.8700 \\
StreamingLLM & 15.8124 & 10.0714 & 3.7500 & 2.3100 \\
D2O & 11.6457 & 3.5005 & 0.3100 & 1.3100 \\
\bottomrule
\end{tabular}
}
\caption{Complete 512-budget single-method scores used for the coarse comparison.
LongBench reports the 21-task macro average, and RULER reports the global average; higher is better.
Quest is shown for completeness but excluded from the best-eviction-single baseline because it is not an eviction method.}
\label{tab:appendix_512_single_methods}
\end{table}
