# Supplementary material for: Exploring a Layer-Wise Design Space for KV Cache Eviction
Source: arXiv:2606.15157 source file (2026-09-17)
Supplement: Supplementary file 4 [file appendix_llama_longbench_budget_sweep_matrix.tex]

\begin{table}[t]
\centering
\small
\setlength{\tabcolsep}{4.2pt}
\resizebox{\linewidth}{!}{%
\begin{tabular}{@{}lrrrrr@{}}
\toprule
Method / configuration & 128 & 256 & 512 & 768 & 1024 \\
\midrule
Full cache & \multicolumn{5}{c}{38.9857} \\
\midrule
\multicolumn{6}{@{}l}{\textit{Single baselines}} \\
CAKE & 32.1214 & 34.6248 & 36.3514 & 36.9890 & 37.5705 \\
CaM & 29.5862 & 31.4490 & 32.7248 & 33.9633 & 34.5600 \\
D2O & 11.9476 & 11.5695 & 11.6457 & 11.9238 & 11.8486 \\
H2O & 29.0733 & 31.3352 & 32.7910 & 33.9533 & 34.7167 \\
PyramidKV & 31.7910 & 34.1567 & 35.8090 & 36.6376 & 37.1414 \\
ScissorHands & 27.1529 & 29.2233 & 31.1881 & 32.0886 & 33.2905 \\
SnapKV & 32.2457 & 34.5805 & 35.9352 & 36.5167 & 36.9905 \\
StreamingLLM & 17.6043 & 16.8233 & 15.8124 & 15.5871 & 15.1319 \\
TOVA & 33.5924 & 34.4814 & 35.6962 & 36.4300 & 37.0571 \\
\midrule
\multicolumn{6}{@{}l}{\textit{PolyKV budget sweep variants}} \\
Method selection only & 35.7476 & 36.8410 & 37.5890 & 37.8690 & 38.0267 \\
Method selection w/ budget allocation & 35.4362 & 36.6681 & 37.7929 & 38.0814 & 38.2181 \\
\bottomrule
\end{tabular}
}
\caption{Complete Llama-3.1-8B-Instruct LongBench budget sweep.
Scores are 21-task macro averages from raw LongBench outputs; higher is better.
Full cache is budget-free and shown once.
Quest is included for completeness but marked as non-eviction.
Method selection only uses \texttt{cosine\_decode} routing with a uniform per-layer budget; Method selection w/ budget allocation keeps the same routing but assigns a non-uniform PPL-sensitivity budget scaled to the target average budget.
Uniform-budget combo is the combo-schema uniform-budget control.}
\label{tab:appendix_llama_longbench_budget_sweep_matrix}
\end{table}
